# Supplementary material for: Faster Subset Selection for Matrices and Applications
Source: arXiv:1201.0127 source file (2013-06-21)
Supplement: Supplementary file 1 [file HC_Appendix_Volume.tex]

\section{Volume sampling for $k \geq n$}

%Our results generalize previous results on volume-based type algorithms
%for the spectral norm version of the problem of Definition~\ref{def:prob}. More specifically, Lemma 3.4
%in~\cite{Pan00} provides a bound for the spectral norm, which is exactly the same as the bound in Theorem~\ref{thm1} for fixed $k=n$.
%This bound can also be obtained via Eqn. 2.4 in Theorem 2.2 in~\cite{HP92}. Our results in the Appendix generalize
%those results to sampling arbitrary $k \ge n$ columns of maximum determinant. Moreover, we prove bounds for both
%the spectral and the Frobenius norm.
%
%The goal of this section is to generalize~\ref{lem:square-expected-by-volume} by showing 
%for samples of size $k \geq n$. Formally, we prove the following lemma.
\begin{lemma}
\label{lem:rect-expected-by-volume}Let $\matX\in\mathbb{R}^{n\times m}$
($m \ge n)$ be a full rank matrix and let $\cal S$ be a random subset
of $[m]$ of cardinality $k$ drawn from $S_{k}(\matX)$. Then,
\[
\Expect{\FNormS{\matX_{\cal S}^{+}}}=\frac{(m-n+1) \cdot \FNormS{\matX^{+}}}{k-n+1}\,.
\]
\end{lemma}

\begin{proof}
%We first introduce a new notation, and state two relevant results. 
%Given a set ${\cal S}$ and $k$ we will use  $\binom{{\cal S}}{k}$ to denote the $k$-subsets of ${\cal S}$.
%We will use the following two intermediate results.
\begin{lemma}[Cauchy-Binet formula.] Let $\matA \in \R^{n \times m}, \matB \in \R^{n \times m}$ and $m\ge n$. Let $|\cal S|$ $=n$.
Then,
$$ \det(\matA \matB\transp) = \sum_{{\cal S} \in \binom{[m]}{n}} \det(\matA_{\cal S}) \det( (\matB\transp)_{\cal S}).$$
\end{lemma}
\begin{lemma}[Lemma 6 in~\cite{GK11}]
\label{GK11-lem6}
Let $\lambda_1 \ge \lambda_2 \ge ... \ge \lambda_m,$ denote the eigenvalues of $\matA \in \R^{m \times m}$. Then,
$$ \sum_{{\cal S} \in \binom{[m]}{r}} \det\left( \matA_{{\cal S},{\cal S}} \right) = \sum_{{\cal S} \in \binom{[m]}{r}} \prod_{i \in {\cal S}} \lambda_i $$
Here, $\matA_{{\cal S},{\cal S}}$ denotes the submatrix of $\matA$ corresponding to row and columns ${\cal S}$.
\end{lemma}
First, notice that,
\[
\FNormS{\matX_{\cal S}^{+}}=\trace{(\matX_{\cal S}\matX_{\cal S}\transp)^{-1}}\,.
\]
A well known formula for the inverse of $\matA$ is $\matA^{-1}=\det{(\matA)}^{-1}\Adj{(\matA)}$,
where $\Adj{(\matA)}$ is the adjugate of $\matA$. We are only interested in
the diagonal values of $(\matX_{\cal S}\matX_{\cal S})^{-1}$ so we need to figure out
only the diagonal values of $\Adj{(\matX_{\cal S}\matX_{\cal S}\transp)}$. Furthermore,
$\matX_{\cal S}\matX_{\cal S}\transp$ is symmetric positive definite so these diagonal
values are always positive. From the definition of adjugate matrix
we find that $i$th diagonal element of $\Adj{(\matX_{\cal S}\matX_{\cal S}\transp)}$ is
exactly the determinant of the matrix that is obtained by deleting the $i$-th row and the $i$-th column
of $\matX_{\cal S}\matX_{\cal S}\transp$. Let $\matY_{i}$ be the matrix obtained by
removing the $i$-th row $i$ of $\matX$. It is easy to see that the matrix obtained
by removing the $i$-th row and the $i$-th column of $\matX_{\cal S}\matX_{\cal S}\transp$ is 
$(\matY_{i})_{\cal S}(\matY_{i})_{\cal S}\transp$. We find that,
\[
\FNormS{ \matX_{\cal S}^{+}}=\frac{\sum_{i=1}^{n}\det{(\matY_{i})_{\cal S}(\matY_{i})_{\cal S}\transp}}{\det{(\matX_{\cal S}\matX_{\cal S}\transp)}}\,.
\]
We can now bound the expected value:
\begin{eqnarray*}
\Expect{\FNormS{\matX_{\cal S}^{+}}} =  \frac{\sum_{{\cal S}\in\binom{[m]}{k}}\det(\matX_{\cal S}\matX_{\cal S}\transp)\FNormS{\matX_{\cal S}^{+}}}{\sum_{{\cal S}\in\binom{[m]}{k}}\det(\matX_{\cal S}\matX_{\cal S}\transp)}
  = \frac{\sum_{{\cal S}\in\binom{[m]}{k}}\sum_{i=1}^{n}\det((\matY_{i})_{\cal S}(\matY_{i})_{\cal S}\transp)}{\sum_{{\cal S}\in\binom{[m]}{k}}\det(\matX_{\cal S}\matX_{\cal S}\transp)}\,.
\end{eqnarray*}
We now observe that
\begin{eqnarray*}
\sum_{{\cal S}\in\binom{[m]}{k}}\det(\matX_{\cal S}\matX_{\cal S}\transp)  \buildrel{(a)}\over{=}  \sum_{{\cal S}\in\binom{[m]}{k}}\sum_{{\cal T}\in\binom{\cal S}{n}}\det(\matX_{{\cal T}}\matX_{{\cal T}}\transp)
 \buildrel{(b)}\over{=} \binom{m-n}{k-n}\sum_{{\cal T}\in\binom{[m]}{n}}\det(\matX_{{\cal T}}\matX_{{\cal T}}\transp)
 & \buildrel{(c)}\over{=} & \binom{m-n}{k-n}\det(\matX\matX\transp)\\
 & \buildrel{(d)}\over{=} & \binom{m-n}{k-n}\prod_{i=1}^{n}\sigma_{i}^{2}\,,
\end{eqnarray*}
where $\sigma_{1},\dots,\sigma_{n}$ are the singular values of $\matX$.
\math{(a)} follows by applying the Cauchy-Binet formula. Also, 
given a set ${\cal S}$ and $k$ we will use  $\binom{{\cal S}}{k}$ to denote the $k$-subsets of ${\cal S}$
\math{(b)} follows from observing that each set in $\binom{[m]}{n}$
is repeated at most $\binom{m-n}{k-n}$ times in the sum.
\math{(c)} follows by applying the Cauchy-Binet formula again.
The equality is again an application of Cauchy-Binet formula.
Finally, \math{(d)} follows from the fact that for symmetric positive-definite
matrices the determinant is equal to the product of
the eigenvalues.

We also have
\begin{eqnarray*}
\sum_{{\cal S}\in\binom{[m]}{k}}\sum_{i=1}^{n}\det((\matY_{i})_{\cal S}(\matY_{i})_{\cal S}\transp)  =  \sum_{i=1}^{n}\sum_{{\cal S}\in\binom{[m]}{k}}\det((\matY_{i})_{\cal S}(\matY_{i})_{\cal S}\transp)
 & \buildrel{(a)}\over{=} & \sum_{i=1}^{n}\sum_{{\cal S}\in\binom{[m]}{k}}\sum_{{\cal T}\in\binom{\cal S}{n-1}}\det((\matY_{i})_{{\cal T}}(\matY_{i})_{{\cal T}}\transp)\\
 & \buildrel{(b)}\over{=} & \sum_{i=1}^{n}\binom{m-n+1}{k-n+1}\sum_{{\cal T}\in\binom{[m]}{n-1}}\det((\matY_{i})_{{\cal T}}(\matY_{i})_{{\cal T}}\transp)\\
 & \buildrel{(c)}\over{=} & \binom{m-n+1}{k-n+1}\sum_{i=1}^{n}\det(\matY_{i}\matY_{i}\transp)\,.
\end{eqnarray*}
\math{(a)} follows by applying the Cauchy-Binet formula.
\math{(b)} follows from observing that each set in $\binom{[m]}{n-1}$
is repeated at most $\binom{m-n+1}{k-n+1}$ times in the sum.
Finally, \math{(c)} follows by applying the Cauchy-Binet formula again.

The matrices $\matY_{i}\matY_{i}\transp$ is equal to the matrix obtained by
deleting column and row $i$ from $\matX\matX\transp$, so according to Lemma~\ref{GK11-lem6}
\[
\sum_{i=1}^{n}\det(\matY_{i}\matY_{i}\transp)=\sum_{i=1}^{n}\prod_{j\neq i}\sigma_{i}^{2}\,.
\]

Finally, we find that
\begin{eqnarray*}
\Expect{\FNormS{\matX_{\cal S}^{+}}}  = \frac{\binom{m-n+1}{k-n+1}\sum_{i=1}^{n}\prod_{j\neq i}\sigma_{i}^{2}}{\binom{m-n}{k-n}\prod_{i=1}^{n}\sigma_{i}^{2}}
  = \frac{\binom{m-n+1}{k-n+1}\FNormS{\matX^{+}}}{\binom{m-n}{k-n}}
  =  \frac{(m-n+1){\FNormS{\matX^{+}}}}{k-n+1}\,.
\end{eqnarray*}

\end{proof}
